# Supplementary material for: Minimal Path and Acyclic Models in the Path Complex
Source: arXiv:2208.14063 source file (2025-05-22)

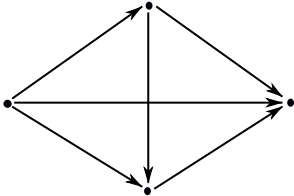

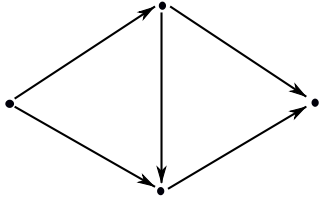

Supplement: Supplementary file 1 [file suppex.pdf]
